# Supplementary material for: XSeg: A Large-scale X-ray Contraband Segmentation Benchmark For Real-World Security Screening
Source: arXiv:2604.03706 source file (2026-04-04)
Supplement: Supplementary file 1 [file appendix.tex]

\section{Appendix Section}
\label{sec:appendix_section}
Supplementary material goes here.
